# Supplementary material for: What distinguishes conspiracy from critical narratives? A computational analysis of oppositional discourse
Source: arXiv:2407.10745 ancillary file (2024-07-15)
Supplement: Supplementary file 1 [file Supplementary_Material_1_-_Filtering_and_Ranking_of_Telegram_Messages.pdf]

# **Methods of filtering and ranking of the Spanish and English oppositional Telegram messages (posts)**

For both languages, the following steps were followed:

1. Filtering of the retrieved messages
2. Ranking according to the post quality

The posts were retrieved from the list of pre-selected telegram channels that tend to contain oppositional messages. After filtering and ranking, top 5000 messages with highest quality index and related to COVID-19 were manually selected, and taken for annotation.

## **1. Filtering of the retrieved messages**

We define a series of criteria to rate each post to maximize the post (telegram message) quality in the final corpus. The set of criteria applied was as follows:

- remove duplicate posts
- remove posts containing null strings
- select only posts whose proportion between non-regular words (like hashtag, links and mentions) and regular ones is lesser than 0.5
- remove posts whose number of words is lesser than 23

## **2. Ranking according to the post quality**

We define 6 criteria to evaluate the posts (telegram messages). These criteria describe properties of the channel and of the post. They are designed to prefer posts that:

- 1) Belong to a channel with a large audience (first criteria).
- 2) A channel where several authors write posts (second criteria)
- 3) A channel where the posts are not written mainly by one author (3rd criteria)
- 4) A channel where the authors have a similar number of posts as average (4th criteria)
- 5) A channel with a great number of post about the topic (5th criteria)
- 6) A post with a sufficient, but not excessive, number of words

### **Criteria 1-5:**

First five criteria are based on the distribution of the post's channel properties and assigned a score according to the property being in the first, second, third, or fourth quartile (distribution is

for the entire dataset, separate for each language). A higher score means a better fit for the criteria (see table 1).

These are the tables that define the quartile-based scores of the posts' channels:

**Table 1. Quartile and scores for the criteria describing the Spanish channels' characteristics**

|                                                                    | Rank of values             | Score |
|--------------------------------------------------------------------|----------------------------|-------|
| <b>Criteria 1. Audience</b>                                        |                            |       |
| 1 Quartile                                                         | Equal or less than 4441,75 | 1     |
| 2 Quartile                                                         | from 4441,76 to 15436,00   | 2     |
| 3 Quartile                                                         | from 15437,01 to 37633,75  | 3     |
| 4 Quartile                                                         | More than 37634,75         | 4     |
| <b>Criteria 2. Authors</b>                                         |                            |       |
| 1 Quartile                                                         | Equal or less than 4,25    | 1     |
| 2 Quartile                                                         | from 4,26 to 17,50         | 2     |
| 3 Quartile                                                         | from 17,51 to 55,50        | 3     |
| 4 Quartile                                                         | More than 55,50            | 4     |
| <b>Criteria 3. Mean of #posts by author</b>                        |                            |       |
| 1 Quartile                                                         | Equal or less than 2,82    | 4     |
| 2 Quartile                                                         | from 2,83 to 7,37          | 3     |
| 3 Quartile                                                         | from 7,38 to 20,46         | 2     |
| 4 Quartile                                                         | More than 20,46            | 1     |
| <b>Criteria 4. standard deviation of the #posts mean by author</b> |                            |       |
| 1 Quartile                                                         | Equal or less than 2,75    | 4     |
| 2 Quartile                                                         | from 2,76 to 13,87         | 3     |
| 3 Quartile                                                         | from 13,88 to 38,23        | 2     |
| 4 Quartile                                                         | More than 38,23            | 1     |

| <b>Criteria 5. Number of posts in the channel</b> |                        |   |
|---------------------------------------------------|------------------------|---|
| 1 Quartile                                        | Equal or less of 70,25 | 1 |
| 2 Quartile                                        | from 70,26 to 206,50   | 2 |
| 3 Quartile                                        | from 206,51 to 480,25  | 3 |
| 4 Quartile                                        | More than 480,25       | 4 |

**Table 2. Quartile and scores for the criteria describing the English channels' characteristics**

|                                                                    | <b>Rank of values</b>      | <b>Score</b> |
|--------------------------------------------------------------------|----------------------------|--------------|
| <b>Criteria 1. Audience</b>                                        |                            |              |
| 1 Quartile                                                         | Equal or less than 2635.50 | 1            |
| 2 Quartile                                                         | from 2635.51 to 12853.00   | 2            |
| 3 Quartile                                                         | from 12853.01 to 34494.00  | 3            |
| 4 Quartile                                                         | More than 34494.01         | 4            |
| <b>Criteria 2. Authors</b>                                         |                            |              |
| 1 Quartile                                                         | Equal or less than 3       | 1            |
| 2 Quartile                                                         | from 3.01 to 7.00          | 2            |
| 3 Quartile                                                         | from 7.01 to 19.25         | 3            |
| 4 Quartile                                                         | More than 19.26            | 4            |
| <b>Criteria 3. Mean of posts by author</b>                         |                            |              |
| 1 Quartile                                                         | Equal or less than 2.33    | 4            |
| 2 Quartile                                                         | from 2.34 to 3.76          | 3            |
| 3 Quartile                                                         | from 3.77 to 12.44         | 2            |
| 4 Quartile                                                         | More than 12.44            | 1            |
| <b>Criteria 4. standard deviation of the posts' mean by author</b> |                            |              |
| 1 Quartile                                                         | Equal or less than 0.62    | 4            |
| 2 Quartile                                                         | from 0.63 to 6.28          | 3            |

|                                                   |                        |   |
|---------------------------------------------------|------------------------|---|
| 3 Quartile                                        | from 6.29 to 14.73     | 2 |
| 4 Quartile                                        | More than 14.74        | 1 |
| <b>Criteria 5. Number of posts in the channel</b> |                        |   |
| 1 Quartile                                        | Equal or less of 10.75 | 1 |
| 2 Quartile                                        | from 10.76 to 48.00    | 2 |
| 3 Quartile                                        | from 48.01 to 115.75   | 3 |
| 4 Quartile                                        | More than 115.76       | 4 |

### Criteria 6:

We define the ideal **number of words (6 criteria)** between 100 and 500 because we observed that a post with less than 100 words tends not to express less personal opinions and only tends to share a link (see table 3).

**Table 3. Criteria (6) of the number of words**

|                           | <b>Score</b> |
|---------------------------|--------------|
| <b>WORDS</b>              |              |
| Between 100 and 500 words | 3            |
| More de 500 words         | 2            |
| Less de 100 words         | 1            |

### Final calculation of the score:

**Finally each post has a score result calculated as an addition of the score in 6 criteria:** audience score+authors score+Medpost score+SD score+number of posts score+Numwords score.

After calculating the scores, we manually select the top 5.000 messages with the highest scores that are **related to COVID-19** for the annotation.
