# Supplementary material for: What distinguishes conspiracy from critical narratives? A computational analysis of oppositional discourse
Source: arXiv:2407.10745 ancillary file (2024-07-15)
Supplement: Supplementary file 2 [file Supplementary_Material_2_-_Selection_of_Words_Promoting_Political_Violence.pdf]

## 1. Prompting the Chat-GPT

We used the `gpt-3.5-turbo-0301` model, configured with a 'context', i.e., a 'system' text whose purpose is to set the context for the model to operate within.

We provide below the English and Spanish contexts, and main prompts fed to the model.

-----

```
ENGLISH_CONTEXT = '''
```

```
You are a social scientist, and you are studying political  
violence. '''
```

```
ENGLISH_PROMPT = '''
```

```
Given a text, list the words that create violent and aggressive  
atmosphere in the text, and that are not necessarily connected  
to physical or sexual violence.
```

```
List only single words, not phrases.
```

```
Format the output as a comma-separated list of words.
```

```
If there are no such words, output 'NONE'.
```

```
TEXT: {text}
```

```
WORDS: '''
```

-----

```
SPANISH_CONTEXT = '''
```

```
Eres un científico social y estás estudiando la violencia  
política.  
'''
```

```
SPANISH_PROMPT = '''
```

```
Dado un texto, elabora una lista con las palabras que crean un  
tono agresivo o violento. No tienen por qué ser palabras  
conectadas con la violencia física o sexual, pueden ser términos  
relacionados indirectamente con la violencia.
```

```
Lista sólo palabras sueltas, no frases.
```

```
Formatea la salida como una lista de palabras separadas por  
comas.
```

Si no hay ese tipo de palabras, pon 'NINGUNA'.

TEXTO: {text}

PALABRAS: ''

## 2. Examples of 'Violent' Texts

**English example of a message that has a high Violence score:**

INTEL - FOXWOLF17 CABLES>China is preparing for WAR<< INSIDE sources say China knows the IMMINENT moment is coming when the U.S. MILITARY will respond against the COVID-19 BIOWEAPON ATTACK<<(inside the PENTAGON Top GENERALS are waiting for the perfect moment to STRIKE... Arrest Treasonous [DS] SPIES in their Military ranks) and government// China is currently positioning Through the WORLD their MILITARY Warships in over 60 countries and plan to take Taiwan soon. >Bidens effort to weaken the Military soldiers by enforcing the vaccines , knowingly well soldiers and military will be divided and a perfect time for China to STRIKE and cause chaos through / SHIPPING STOPPAGE. ENERGY CRISES../ ESSENTIAL SUPPLIES.. All MILITARY is on high ALERT >>>DEEP STATE CABAL In every country is Working hard together to stop the 32 NATION ALLIANCE MILITARY from stepping in and stopping the Depopulation agenda that is connected to resetting the financial system( every time the deep state money goes into major debt..[they] create wars / their financial institutions can not sustain growing societies.. That's why WAR is created every time their financial system starts to [CRASH]///) [THEY] are starting to with hold energy resources/ <<< this will bring the collapse [CRASH] THE DEEP STATE plan is crumbling at many LEVELS and[EXPOSURE] is leaking and time is ticking..... There is only one chance for all MILITARY ALLIANCE to STRIKE together on their own deep state governments and [DS] MILITARY CCP CHINA KNOWS THIS MOMENT IS COMING<< WITHIN CHINA IS A SILENT COUP HAPPENING ALSO .. ALL COUNTRIES ARE ON HIGH ALERT.... >>DARK WINTER<< \_\_\_ Many of you are very unaware.. 1.4 Billion humans will die from the vaccines ( Bioweapon attack)and the death counts chaos has already started/// These important Chess moves happening had to happen .. White HATS took a step back as the enemy used up their final moves and energy..... Then the STRIKE HAPPENS<< THE NEWS IS FAKE THE WAR IS REAL / \_\_\_\_\_ when I say [FAKE] WAR ..I mean the DEEP STATE is planning these WARS across the world for confusion.. To have the sheep look away from the Truth of[EXPOSURE] of the Plandemic. The Bioweapon vaccines... This[FAKE] WAR is never the less a WAR..... But the WHITE HATS MILITARY will step

in before MAJOR Nuclear conflict erupts into a holocaust <<<< \_\_\_\_ It's always important to have your 30\_60 days of food, water and supplies ready .. Common sense< \_\_\_\_ [CRASH] Your your inside this\_EVENT NEAR DEATH CIVILIZATION EVENT YOUR INSIDE THIS EVENT... \_\_\_\_ INSIDE THE STORM \_\_\_\_ PAIN \_\_\_\_  
@QNewsOfficialTV

### **Spanish example of a message that have a high Violence score:**

¿ERES ESPAÑOL? REENVÍA ESTO EN TUS GRUPOS. El gobierno de España, con el dinero de todos los españoles (es decir, con tus cientos de impuestos te esclavizan, ya que somos el país desarrollado con más impuestos del mundo), y aprovechándose como YENAS de nuestro trabajo y del sudor de nuestra frente, envía armas a UCRANIA SIN CONSULTARNOS, ARMAS PAGADAS CON NUESTROS IMPUESTOS Y A FONDO PERDIDO. PÁSALO, TÚ PUEDES CAMBIAR LAS COSAS=><https://t.me/supercontagadores/10038> Lo que está ocurriendo (a pesar de que tú no lo veas en la TV judía y los periódicos judíos), es que con esas ARMAS que ESPAÑA ENVÍA a UCRANIA (recordad el NO A LA GUERRA con AZNAR e Irak, y pensad porqué no sale ahora todos esos "artistas" que llenaron las calles de España con el "no a la guerra", con el símbolo del OJO DE HORUS, con el OJO MASÓNICO), los NAZIS CONFESOS del batallón Azov de Zelensky, comete crímenes de LESA HUMANIDAD contra CIVILES. Bulgaria y Hungría se niegan hasta ahora a entregar armas a Ucrania al ver los CRÍMENES de lesa humanidad que están cometiendo, pese a ello, la gran mayoría de países europeos, sí CEDEN, debido a que CEDEN a las EXIGENCIAS de américa. Imaginaos que España lo hace al revés, sabe que en IRAK no hay armas de destrucción masiva, y envía armas a IRAK. Todo es geopolítica y los americanos siguen siendo LOS (satánicos) AMOS DEL MUNDO. Sánchez, sólo es un títere que hace lo que dice américa. Le envían allí los DUEÑOS DEL MUNDO como símbolo de sumisión de ESPAÑA (que fue un imperio donde no se ponía el sol), al Nuevo Orden Mundial satánico. Y del mismo modo que nos dejamos robar el oro de moscú, ahora dejamos que se cometan CRÍMENES DE GUERRA Y DE LESA HUMANIDAD CON NUESTRAS ARMAS y CON NUESTRA MARCA. ES COMO SI LO HICÉSEMOS NOSOTROS. Sacar a FRANCO del Valle de los caídos fue un RITUAL SATÁNICO. Todo esto es SIMPLE Y PURA HUMILLACIÓN de España sometándose al NOM. Los Goyim deben saber quién manda realmente en el mundo. Es un claro mensaje de fuerza al mundo, para que se sepa quién manda en el mundo en realidad: La élite satánica de EEUU. Los Ucránicos MATAN, humillan, torturan, y someten a SERES HUMANOS (civiles o militares), con NUESTRAS ARMAS. Después, como controlan todos los medios de comunicación, dan la vuelta a la tortilla, y culpan a RUSIA. Nuestro PELELE del NOM Sánchez, ha cumplido misión haciéndose ver en

Ucrania. Todo para que los NAZIS a las órdenes de la mariconada de ZELENSKY, sigan cometiendo CRÍMENES DE GUERRA (disparando a prisioneros) y CRÍMENES de LESA HUMANIDAD (utilizando a población civil como escudos humanos). Todo lo hace por SUS COJONES el DICTADOR PEDRO SÁNCHEZ, Y SIN PREGUNTAR AL PUEBLO ESPAÑOL QUÉ LE PARECE. Y eso que que "SUPUESTAMENTE" el pueblo español en su carta magna (la constitución redactada en una logia masónica), dice en su artículo primero que EL PUEBLO ES SOBERANO (La soberanía nacional reside en el pueblo español, del que emanan los poderes del Estado.) Pese a todo esto, y a pesar de tener claramente un TÍTERE del NOM como presidente del gobierno, los españoles creen (o mejor dicho, quieren creer para no afrontar la realidad) que "viven en democracia". A estas alturas me dais mucho asco, mucha pena, incluso os considero DEFICIENTES MENTALES, a los que seguís llamando a FRANCO DICTADOR y llamáis a esto que llevamos dos años padeciendo "DEMOCRACIA". Lo peor de todo, ha sido el lavado de cerebro con la "VACUNA" (reconocido experimento génico), y el BOZAL de la esclavitud. Mucha gente en España, sigue CREYENDO por FE, que vacuna y el BOZAL han servido, o sirven para algo. Da igual que seas policía, guardia civil, funcionario, empresario, empleado, parado o seas un ser vivo y no una persona: Si te has puesto BOZAL o te has vacunado, te has HUMILLADO y te has SOMETIDO al Nuevo Orden Mundial. Y lo peor está por llegar, porque como ya saben que eres fácil de MANIPULAR Y SOMETER, volverán a hacerlo cuando quieran. Simplemente... ¡¡¡DI NO!!! Sigue=><https://t.me/supercontagiadores/10039>  
@supercontagiadores

### 3. Lists of 'Violent' Words

#### ENGLISH:

abandon

abandonment

abet

abnormal

abnormally

abuse

abuser

accomplice

accuse

acrimony

addictive

afraid

aggression

aggressive

agitate

agitation

alarm

alarming

alert

alien

ally

ammunition

amnesty

anarchist

anarchy

animosity

antichrist

anunnaki

apocalyptic

appalling

arbitrary

armament

army

arrest

arrogance

assassin

assassinate

assault

assaulter

asshole

atrocities

attack

authoritarian

authoritarianism

backfire

ban

bananafrance

bananagermany

bananauk

bankrupt

barbarian

barbaric

baseless

bastard

batshit

battle

battlefield

beast

beat

belittle

bellicose

belligerent

berserk

betray

bias

bigotry

bioterrorist

biowarfare

bioweapon

bite

bizarre

blackmail

blame

blasphemy

blast

blaze

bogus

boogeyman

bot

boycott

boycotts

brainwash

brutal

brutality

brute

buffoon

bullshit

bully

burglary

burn

captivity

capture

cartel

catastrophe

catastrophic

caution

censor

censorship

censure

chaos

chaotic

charade

chattle

chauvinist

cheat

chicom

chimeras

clandestine

clash

clown

coerce

coercion

coercive

collapse

colonize

combat

combative

commando

complicit

con

conceal

condemn

confidential

confiscate

contaminate

contamination

convict

corrupt

corruption

coup

covert

coverup

crackdown

crap

crash

crazy

creed

creepy

crime

criminal

criminality

crook

crucify

cruel

cruelty

crush

crusty

cull

curse

daemon

daemon

damage

damnation

danger

dangerous

deceit

deceitful

deceive

deceiver

deception

defeat

defiance

demolition

demon

demonic

demonization

demonolatry

deplorable

depopulate

depopulation

deprive

derail

desperate

desperation

despot

destroy

destruction

destructive

detain

detainee

devastating

devastation

deviant

devil

diabolical

dictator

dictatorship

diddle

diktat

disaster

discredit

discriminate

discrimination

discriminatory

disenfranchise

disguise

disgusting

dishonorable

disingenuous

dismantle

disrupt

disruption

dissident

distort

disturb

doctrine

dodge

dogma

doomster

doxxe

draconian

dramatic

dread

dumb

dumbest

dumbfuck

dumbly

dupe

dystopia

dystopian

eerie

eff

endanger

endgame

enemy

enforce

enmity

enslave

enslavement

entice

envy

erratic

eugenic

evil

explode

explosion

explosive

exterminate

extermination

extinction

faggot

fallacy

fallout

falsely

falsify

fanatic

fear

fearful

ferocious

fightback

filch

filth

filthy

fire

flame

flammable

foist

fool

foolish

forfeit

fraud

fraudulent

freak

freakshow

frightening

frustrate

frustration

fuck

fucking

furious

fury

gaffe

gag

gang

garbage

gaslight

gaslighte

gaslit

gatekeeper

genocidal

genocide

ghoulish

gimmick

grift

grim

grimmer

guerrilla

guilty

guise

gullible

gun

gunman

hallucination

harm

harmful

hate

hateful

hater

hatred

heinous

heist

hell

herd

heretic

hijack

hitlist

hoax

holocaust

homicide

homophobe

homosexual

hopeless

horrible

horrific

horror

hostage

hostile

hostility

hubristic

humiliate

hypnosis

hypnotist

hypocrisy

hypocritical

idiot

idiotic

ignorant  
illegal  
immoral  
implode  
imprison  
imprisonment  
incendiary  
incestuous  
incite  
inciteful  
incitement  
incriminate  
indignity  
indoctrinate  
indoctrination  
ineffective  
inequity  
infiltrate  
infiltration  
inhumane  
injure  
innundate  
inquest

insane

insanely

insanity

insatiable

instability

instigation

instill

insult

insurgency

insurrection

internment

intimidate

intimidation

intrusive

invasion

islamophobe

jail

jeopardy

jingoist

judge

kill

killer

killers

killling

lame

laughable

launder

lawlessness

lawsuit

leech

liar

libtard

lie

lobby

lobbyist

loom

luciferian

mad

madness

mafia

maim

malice

maniac

maniacal

manipulate

manipulation

massacre

mayhem

menace

mercenary

merciless

mercilessly

mess

messy

militant

militarize

military

militia

miserable

mislead

mockingbird

mommy

monster

monstrous

morality

moronic

murder

murderer

murderous

mutiny

nasty

nazi

nazism

neanderthal

nightmare

nonce

nonsense

normie

oath

obscene

obstruction

occult

occultist

offend

offender

ominous

opportunist

oppression

orchestrate

orwellian

ostracise

outcast

outrage

outrageous

overload

overthrow

overturn

panic

panopticon

paramilitary

parasite

pathetic

peasant

peddle

pedophile

pedophilia

penalise

penalty

peril

perilous

perpetrate

perpetrator

persecute

persecution

perverse

pervert

phony

pilfer

pimp

placard

placebo

plaintiff

pliable

plummet

plutocracy

poison

poisoner

poisonous

police

policy

pollute

pollution

preach

precautionary

predatory

prejudice

pretend

primate

propaganda

propagandist

prostitute

protest

protester

pseudoscientist

psychiatric

psychopath

psychotic

psyop

pugnacious

punish

punishment

puppet

puppetdom

quack

racism

racist

racket

rage

raid

rally

rampage

rapacious

rape

rash

rebel

rebellion

rebellious

recklessly

relentless

renegade

repugnant

resentment

resist

resurgence

retaliation

retard

revenge

revolt

revolution

revolutionary

rhetoric

ridiculous

rigour

riot

risk

risky

rogue

ruthless

sabotage

sadistic

sarcastic

satan

satanic

satanist

savage

scam

scamme

scapegoat

scare

scary

scream

screw

scum

scumbag

secret

secretly

sedition

selfish

separatist

serpent

sexist

shamble

shame

shameful

shamelessly

shapeshifte

shark

sheep

shill

shit

shite

shithole

shitlib

shitshow

shittily

shock

shocker

shockingly

shooting

shot

shyster

simulate

simulation

sinful

slam

slant

slaughter

slave

slavery

slur

smash

smuggle

snake

sneaky

snooty

sociopath

soldier

sordid

soulless

spite

spy

squash

stab

stalker

startling

starvation

starve

steal

sting

stolen

stooge

storm

stranger

strike

stupid

stutter

submissive

subpoena

subversion

subversive

subvert

sue

supremacist

surge

surreptitious

suspect

tactic

tamper

taunt

terrible

terrify

terror

terrorism

terrorist

terroristic

terrorize

threat

threaten

throttle

throw

thug

thwart

torture

totalitarian

totalitarianism

toxic

toxicity

traffic

trafficker

tragedy

tragic

traitor

transphobe

traumatize

travesty

treason

treasonous

tremor

trial

tribunal

trick

triumph

trojan

troop

turmoil

tyrannical

tyranny

tyrant

undermine

unethical

unlawful

unlawfully

unlicensed  
unrighteous  
unsafe  
upheaval  
useless  
vengeance  
venom  
vermin  
vertigo  
vicious  
vile  
vilify  
villain  
violate  
violation  
violence  
violent  
vitriol  
war  
warfare  
warlike  
warlord  
warp

warroom  
wartime  
wasteland  
weapon  
weaponise  
weaponize  
wetwork  
whacka  
whistleblower  
wicked  
worthless  
wreck  
xenophobe  
zealot  
zionist  
zombie

**SPANISH:**

abandonar  
aberración  
aberrant  
aborrecible

aborregado

abrumado

absurdez

absurdo

abusar

abuso

acosándome

acusado

acusar

adoctrinado

adoctrinamiento

agitar

agredido

agredir

agresión

agresivo

alambrado

alarmar

alarmar él

alarmista

alertar

alevosía

alucinado

amedrentándol

amenaza

amenazado

amenazando él

amenazar

angustiar

aniquilado

aniquilar

anormal

apartheid

apestado

aplstar

apocalíptico

apresamiento

arbitrariedad

arbitrario

arma

arrestar

arresto

arruinarlo

arsenal

artimaña

asalto

asesinado

asesinar

asesinato

asesino

asqueroso

astucia

asustado

atacar

ataque

atemorizarno

atentado

aterrador

aterro

aterrorizar

atrapado

atrocidad

atropellado

aullador

autoritarismo

avaricia

avergonzar él

avergonzarno

banear

barbaridad

barbarie

bastardo

basura

batalla

bebelejía

bestia

boicot

boicotear

bomba

bombazo

boom

borrego

bramar

broncar

bruja

brutal

brutalidad

burla

burlar

burlar él

calumnia

caos

capitulación

casta

castigado

catástrofe

catastrófico

cautivo

cegato

ceguera

censura

censurado

censurar

chantaje

chantajeándol

chantajear

chantajista

chimpacé

chusma

cínicamente

circo

coacción

coaccionado

coaccionándol

coaccionándon

coaccionar

coactivo

coartar

cobarde

codiciar

coercitivo

colaboracionista

colapsa

colapsar

colapso

colusión

combatido

combatiente

combatir

cómplice

coñazo

confiscación

conquistar

contaminación

contaminado

contaminante

contaminar

controlador

corrupción

corrupto

crimen

crimén

criminal

criminalizar

crueldad

cuchilla

cuchillo

culpa

culpabilidad

culpable

culpar

ddt

decomiso

defender

defensa

defensor

degeneración

delictivo

delincuente

delirio

delito

demandado

demoledor

demoniaco

demonio

demonización

denostar

depredadorar

derribo

derrocado

derrota

derrotado

desamparado

desarmar

desastre

desbaratar

descaro

desesperación

desesperado

desfalcador

desgarrar

deshumanización

deshumanizadora

desmesurado

desmoronar

desnazificar

desobedecer

desobedecerl

desobediencia

desolación

desperado

desplomar

despoblación

despotricar

desprestigiarno

desproporcionado

destap

destapa

destapado

destrozar

destrozo

destrucción

destruido

destruir

destruirno

desvirtuar

dictador

dictadura  
difamación  
discrimín  
discriminación  
discriminar  
discriminatorio  
disfrazado  
disidencia  
disidente  
disimular  
disparar  
disparate  
distópica  
disturbio  
dominar  
dominio  
draconiano  
drama  
dramática  
drásticamente  
egoísta  
ejecutor  
elitista

embargo

embustero

encubiertar

encubierto

encubrimiento

encubrir

enemiga

enemigo

engañado

engañar

engañar yo

engaño

engañosa

engñoso

engendro

envenenado

envenenamiento

envenenar

envidia

escalofriante

esclavitud

esclavizar

esclavizarno

esclavo

esconder

esconder él

escupir

espada

espeluznante

espía

esposar

estafa

estafador

estafar

estallar

estupidez

estúpido

eugenésico

eugenesis

eugenista

eugenista

excluir

explosivo

exterminar

facha

falacia

falsario

falsear

falsedad

falso

fanatismo

farsant

farsante

feo

ficticio

filtración

flagrante

flipado

fraude

fraudulento

fugar

furioso

fusilamiento

ganado

genocida

genocidio

genocido

gerontocidio

gilipol él

grave

guerra

guerrero

hambruna

herido

hijosdelagranputa

hipnotizado

hipocresía

histeria

holocausto

homicidio

horror

horroroso

hostiar

hostil

hostilidad

humillación

humillado

humillante

humillar

humillarnos

humille

hundir

idiota

idiotéz

ignominia

ignorante

ilegal

ilegalidad

imbécil

impune

impunidad

incautado

incompetente

incultar

inculto

indemnización

indigno

inepto

inexperto

infame

infamio

infiltrado

injerencia

injusto

inmaduro

inmoral

inocente

inquietante

inquisición

insultar

insultar él

insulto

intimidación

intimidado

intimidar

inútil

invadido

invasión

ira

irracionalidad

joder

jodido

judicial

juez

juicio

justicia

juzgada

juzgar

lacayo

ladrón

lameculo

levantamiento

llamamiento

lobbi

loco

locura

machacar

mafia

maldad

maldito

maligna

maligno

malísimo

maltratado

malvado

manicomio

manipula

manipulación

manipulado

manipular

manipulativa

maquillar

masacre

matadero

matado

matanza

matar

matar él

matarrata

matir

matrix

mediocr

menospreciar

mentido

mentir

mentira

mentirosa

mentiroso

merluzo

miedo

mente

mierdo

militar

miserable

moral

moralidad

multa

multado

narcopatrón

navaja

nazi

nazitario

nefasta

negligente

ninguneado

ningunear

obcecado

obsesión

obsoleta

obsoleto

obstruccionista

odiar

ofender

ostia

pánico

pantomimo

paparrucha

paranoia

parásito

patético

payaso

pedofilia

pelear

peligro

peligrosidad

peligroso

peligrsidad

penal

perpetrador

perrodista

persecución

perturbado

peste

pijo

piratear

pisotear

porculera

premeditación

presionado

presionar

prevaricación

prisionero

propaganda

propagandista

provocación

psicópata

puñalado

puñetero

purga

puta

puto

quemado

quemar él

quintacolumnista

rabiar

racista

rata

rebelión

recochineo

rendáis

rendición

represor

reprimir

reptil

resistencia

rezagado

ridículo

riesgo

robar

ruina

saboteada

sanción

sancionar

sangrante

saqueado

sataná

satánica

satánico

satanismo

secretismo

secreto

secta

sectaria

secuestrado

secuestrador

secuestro

sensacionalismo

sentencia

shock

silenciar

simplista

simulación

simulacro

sinistra

sinvergüenza

sobornado

soborno

sobredimensionar

sobresueldo

sociopata

soldado

sometimiento

sospechoso

subversión

subyugar

sucumbir

suicidacer

sumisión

supervivencia

superviviente

supremacista

táctico

tapadero

tapar

temblor

temer

temeridad

temor

tergiversar

terrible

terriblemente

terror

terrorífico

terrorismo

terrorista

timo

tiranía

tiránico

tiranir

tiroteo

títere

tonto

torturado

torturar

totalitaria

totalitario

totalitarismo

traición

traicionar

traidor

trampa

trampeado

traumatizar

trinchera

trolar

trucar

tsunami

turbia

veneno

venenoso

vergüenza

vileza

vilipendiado

violabilidad

violación

violar

violencia

violentar

violento

vulneración

vulnerar

yonquis

zombie
